# Supplementary material for: Topographic control of order in quasi-2D granular phase transitions
Source: arXiv:2108.07518 ancillary file (2021-08-17)
Supplement: Supplementary file 1 [file SupplementaryInformationJGDowns2021.pdf]

# Supplementary Information

*"Topgraphic control of order in quasi-2D granular phase transitions"*

J.G. Downs, N.D. Smith, K.K. Mandadapu, J.P. Garrahan, M.I. Smith

## Methods

Our experiments use metal base plates that were prepared with two different surface topographies: the first flat and the second with a triangular array of dimples. Both plates are constructed from 10mm thick Aluminium and are slightly roughened through sandblasting. The triangular array of dimples uses a spacing of L ~ 4.62mm (see diagram, dimples in red). The dimples are cut 0.13mm deep with a precision CNC machine using a 10mm diameter spherical cutter. This leads to dimples over the entire surface of the plate with a radius of 1.15±0.05mm as illustrated in supplementary figure 1. The diameter of both types of particles is 4mm.

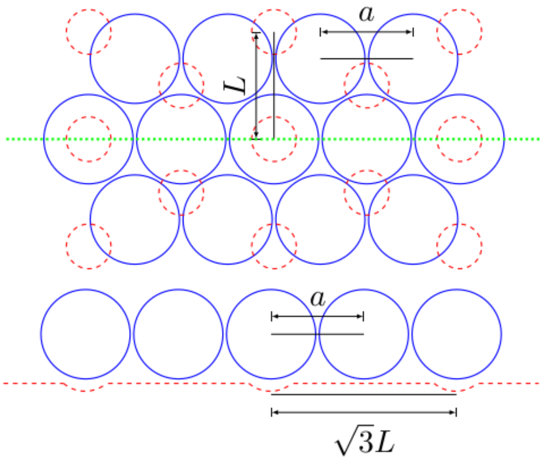


*Figure S1: Schematic of the crystal phase on the dimpled plate. (Top) Diagram, from above, showing the arrangement of the particle's crystal phase (blue circles) above the triangular lattice of dimples (red dashed circles). L is the spacing between the dimples and a is the spacing between the particles. (Bottom) Diagram, from front, along the plane of the dashed green line.*

The metal base plates used in the experiment are mounted on leaf springs above an electromagnet. The electromagnet causes the plate to move up and down sinusoidally. Before experiments are started, the shaker and its water cooler are turned on for one hour to allow the temperature of the electromagnet to stabilize. The acceleration provided by the magnet at different powers was tested and found to be repeatable through heating/cooling cycles and through long steady state experiments.

The experiment is mounted on motorized legs, which enable precise software controlled levelling. Levelling is achieved by tracking the positions of particles and changing the height to remove any bias. The system can be levelled with either the completely orderphobic or completely orderphillic boundary in place. When the orderphobic boundary is in place then the system is repeatably cooled from high to low $\Gamma$ such that a crystal forms. The crystal tends to sit on the 'downhill' side so the

motorized legs are raised on the side of the crystal. When the orderphillic boundary is in place then a bubble of liquid forms in a crystal phase, this bubble sits on the 'uphill' side so the legs are lowered on the crystal's side. Since the crystal / bubble may nucleate at any point in the tray we perform many such cooling and heating cycles and determine the average position before the software adjusts the motorized legs to try and level the system. This is repeated until the average position of the crystal / bubble sits at the center of the tray. Once the system has been levelled, the amplitude is increased so that the entire system is in the liquid phase prior to beginning each experiment. It's important to note that when the system is flat the position of the bubble randomly forms around the cell away from the center, however the average position of the bubble is central.

The particles are 4mm diameter black nitrile balls with a shore hardness of 70A. The coefficients of restitution were estimated by filming particles dropped from a known height onto a flat surface. The coefficient of restitution between the particles and the aluminum base plate is $\sim 0.1$. The red polypropylene particles shown in Figure 1b of the paper have a coefficient of restitution with the steel base plate of 0.6. The particle-particle coefficient of restitution ($e_{pp}$) is difficult to measure but an estimate can be obtained by dropping each type of particle onto either a similar rubber sheet for the nitrile particles or a sheet of polypropylene for the polypropylene particles. This gives $e_{pp} \sim 0.03$ for the nitrile particles and $e_{pp}$ ~ 0.6 for the polypropylene respectively. The particle-wall coefficient will be similar to $e_{pp}$ for the nitrile particles but is again extremely low for the polypropylene particles dropped onto the rubber sheet, $e_{pw}$ ~ 0.03.

## Arrangement of the crystal phase

A crystal phase can form whenever the particle area fraction exceeds a critical value corresponding to a particle number that exceeds the number of dimples ($\phi > 0.585$). The crystal phase that forms on the dimpled plate is not the 1x1 commensurate lattice (where each dimple has a particle directly above it), instead a $\frac{\sqrt{3}}{2}R30°$ lattice forms where the crystal phase is rotated by 30 degrees relative to the dimple lattice and is more tightly spaced so that there are 2 particles per dimple in this direction, as seen in Figure S1.

## Hysteresis

Hysteresis experiments were also performed at rates slower than the rates shown in the paper. Figure S2, shows experiments conducted at ($\dot{\Gamma} = 0.0013, 0.0026$ & $0.0052\ s^{-1}$). Rates higher than $\dot{\Gamma} = 0.0052\ s^{-1}$ were not analyzed as at these rates the system is quenched and a fully ordered state is not reached.

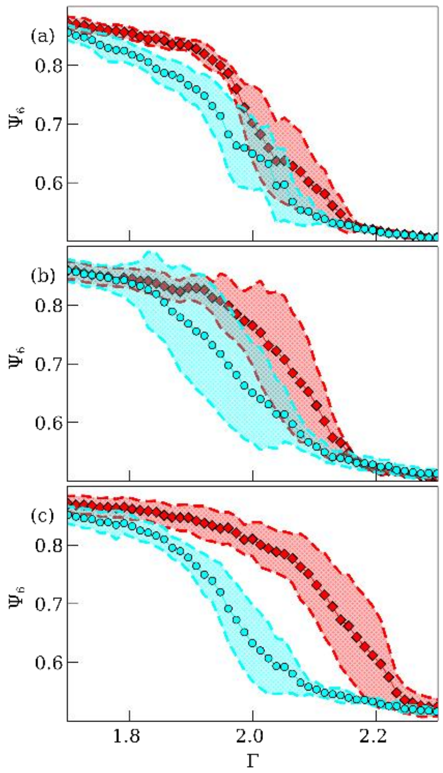


*Figure S2: Hysteresis of the hexatic order parameter on a dimpled plate. Cooling and heating at rates of a)* $\dot{\Gamma} = 0.0013$ *b)* $0.0026$ *c)* $0.0052 s^{-1}$ *showing increasing hysteresis with cooling rate.*

Experiments were also repeated using the flat plate, which showed a lack of hysteresis when cooled, irrespective of rate (Figure S3). This is consistent with a continuous transition.

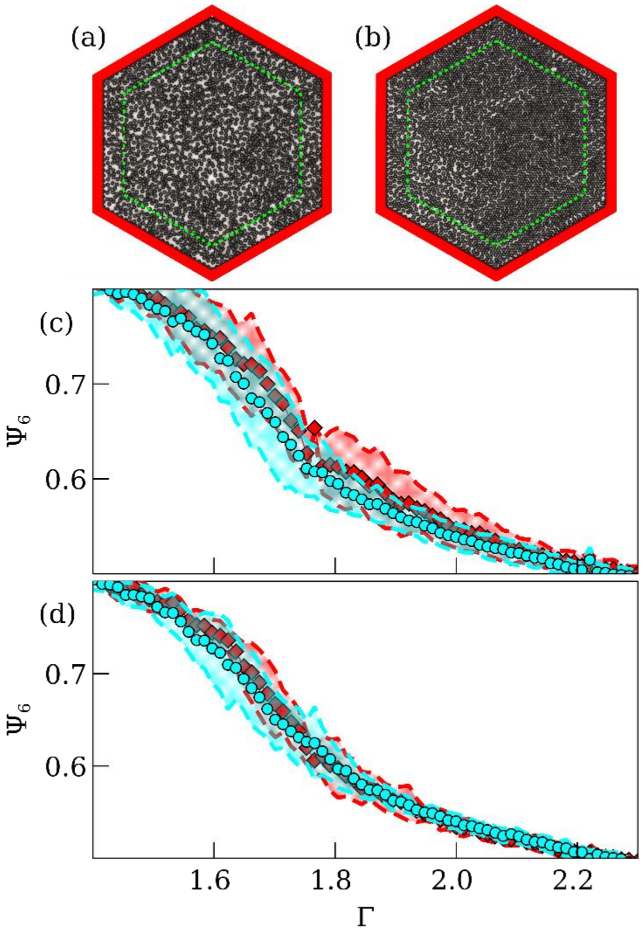


*Figure 3: Figure demonstrating the absence of hysteresis while moving through the liquid-solid phase transition on a flat plate. (a) High $\Gamma$ starting condition of the system. (b) Low $\Gamma$ end position of the system. Only particles inside the green line are considered for analysis. (c) Cooling (blue circles) and heating (red diamonds) curves for a cooling/heating rate of $\dot{\Gamma} = 0.0026\ s^{-1}$. (d) Cooling and heating curves for a rate of $\dot{\Gamma} = 0.0052\ s^{-1}$. Shaded regions show the standard deviation between the 5 repeat experiments.*

## Calculating the translational order parameter

The translational order parameter for particle $j$ is given by $\psi_T = e^{i\vec{G}\cdot\vec{r}_j}$, where $\vec{r}_j$ is the position vector of particle $j$ and $\vec{G}$ is a primary reciprocal lattice vector. This is extremely sensitive to both the length and angle of $\vec{G}$, which in an experimental system, are not trivial to calculate as the orientation and size of the system are not automatically known.

To achieve this, a Delaunay triangulation of the particles in the solid phase is calculated which draws lines between neighbouring particles in the triangular lattice such that no particle is in the circumcircle of any other. This returns a list of all the vectors between neighbouring particles.

A histogram of all the vector angles is then calculated which will have a peak for each of the three directions. The median value of data around one of the histogram peaks is taken as the angle of the lattice vector. The length of the lattice vector is taken as the median length of all the vectors. Given the angle and length of the lattice vector $\vec{a}$ the reciprocal lattice vector $\vec{G}$ is then calculated where $\vec{G}_r = \frac{4\pi}{\vec{a}_r\sqrt{3}}$ and $\vec{G}_\theta = \vec{a}_\theta + \frac{\pi}{2}$.

# Supplementary Movies

Supplementary movie 1 shows the formation of critical nucleus as the system is cooled ($\phi \sim 0.84$). The particles are color coded according to the value of the hexatic order parameter (Blue high order, Red low order).

Supplementary movie 2 shows an animation of the orientational and translational order parameters, plotted as vector fields for the dimpled plate. The global susceptibility is also plotted as a function of the dimensionless acceleration. The current acceleration of each vector field image is indicated by the dotted green line.

Supplementary movie 3 shows an animation of the orientational and translational order parameters, plotted as vector fields for the flat plate. The global susceptibility is also plotted as a function of the dimensionless acceleration. The current acceleration of each vector field image is indicated by the dotted green line.
